# Supplementary material for: Evaluating Correctness and Faithfulness of Instruction-Following Models for Question Answering
Source: arXiv:2307.16877 source file (2024-04-17)
Supplement: Supplementary file 1 [file appendix_metric_failures.tex]

\section{Failure Cases of Metrics}\label{appendix_sec:metric_failures}

\paragraph{Lexical-based metrics}
\label{paragraph:lexical_based_metrics_failures}
% \Cref{fig:correctness_error_analysis} presents an overview of the F1 metric failures; the exact percentages and counts can be found in \Cref{tab:appendix_stats_model_failure}.

\paragraph{GPT4-Eval}
\label{appendix_sec:gpt4-eval-failure}
To better understand how GPT4-Eval fails compared to F1, we took the subset of annotated failure cases (described in \Cref{paragraph:correctness_error_analysis}) where GPT-4Eval also predicts 0; In total, we found 70 instances out of overall 296 samples. \Cref{fig:subset_failure_categories_gpt4} shows the distribution of failure subcategories for the GPT-4Eval subset. We observe that a higher proportion of failures are caused by open-ended questions, whereas more elaborated answers and enumeration of reference answers are less penalized by GPT4-Eval compared to the remaining failures. Moreover, all other subcategories now have a higher proportion due to the gap left by more elaborate answers and enumeration of reference answers. To illustrate the new findings, we include a few samples in \Cref{fig:appendix_gpt4_failure_examples}.

\begin{figure*}[th!]
    \centering
    \includegraphics[width=\linewidth]{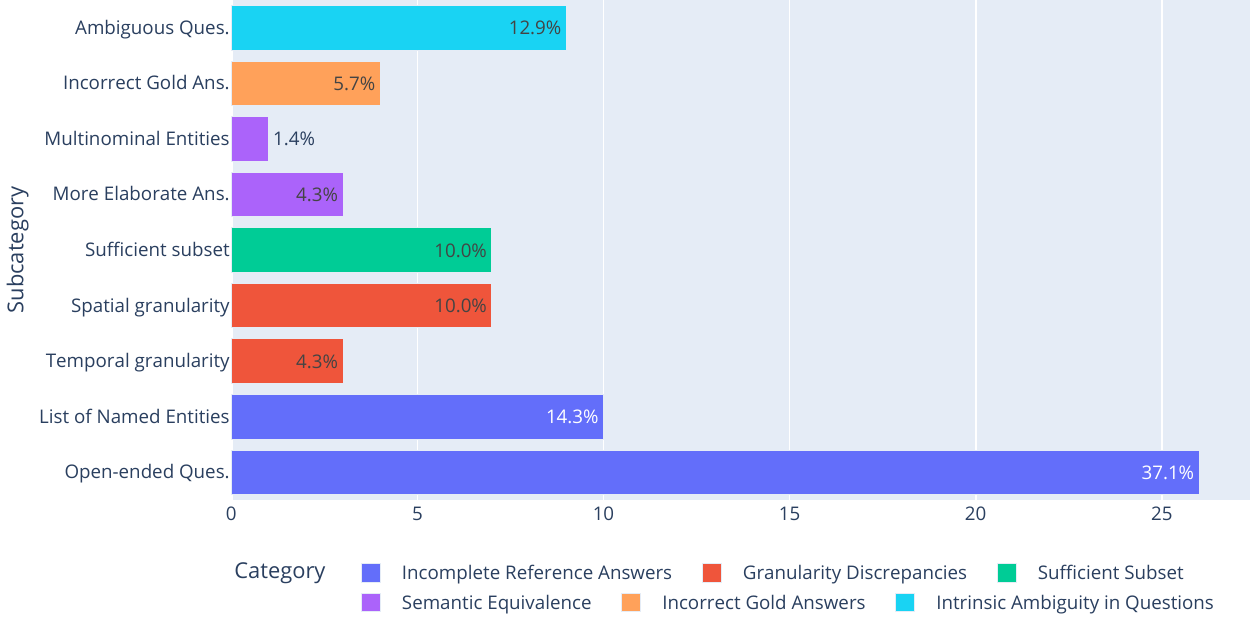}
    \caption{Distribution of failure cases of GPT4-Eval by sub-category. It struggles the most with \textit{Open-ended Questions}.
    }
    \label{fig:subset_failure_categories_gpt4}
\end{figure*}
\begin{figure*}[t]
\small
\begin{tabular}{p{2\columnwidth}}
\toprule
\textbf{Error Type:} Incomplete Reference Answers - Open-ended Questions\\
\textbf{Dataset}: TopiOCQA \\
\\
\textbf{Question}: does she (J.K. Rowling) donate to any charity? \\
\textbf{Reference answer}: Yes - In 2002, Rowling contributed a foreword to ``Magic'', an anthology of fiction published by Bloomsbury Publishing, helping to raise money for the National Council for One Parent Families. \\
\textbf{Alpaca's response}: Yes, she does. She is a member of both English PEN and Scottish PEN, and has donated the proceeds from several of her books to various charities.\\

\midrule

\textbf{Error Type:} Incomplete Reference Answers - List of Named Entities\\
\textbf{Dataset}: Natural Questions \\
\\
\textbf{Question}: what kind of animals live in the great victoria desert \\
\textbf{Reference answer}:  malleefowl; water-holding frog; great desert skink; sandhill dunnart; dingo; sand goanna; crest-tailed mulgara; southern marsupial mole; chestnut-breasted whiteface; perentie\\
\textbf{Flan-T5's response}: lizard.\\

\midrule

\textbf{Error Type:} Intrinsic Ambiguity in Questions\\
\textbf{Dataset}: Natural Questions \\
\\
\textbf{Question}: who played in the stanley cup finals last year\\
\textbf{Reference answers}: Nashville Predators, Pittsburgh Penguins\\
\textbf{GPT-3.5's response}: The Washington Capitals and the Vegas Golden Knights played in the Stanley Cup Finals last year (2018).\\
% clarifying question
% id 966
\bottomrule
\end{tabular}
\caption{Examples where GPT-4Eval predictions differ from human judgement (alongside $F_1<0.3$). %More details in \Cref{appendix_sec:gpt4-eval-failure}.
}
\label{fig:appendix_gpt4_failure_examples}
\end{figure*}
