# Supplementary material for: Evaluating Correctness and Faithfulness of Instruction-Following Models for Question Answering
Source: arXiv:2307.16877 source file (2024-04-17)
Supplement: Supplementary file 2 [file appendix_unanswerability.tex]

\section{Failure Cases of Models in Faithfulness w.r.t Irrelevant Knowledge}
\label{appendix_sec:unanswerability}
\begin{figure*}[ht!]
\small
\begin{tabular}{p{2\columnwidth}}
\toprule

\textbf{Dataset}: NQ \\
\\
\textbf{Question}: points on a sphere or angles in a circle are measured in units called \\
\textbf{Reference answer}: radians\\
\textbf{Responses}:\\ 
\textbf{Alpaca}: \textcolor{purple}{radians}\\
\textbf{Flan-T5}: \textcolor{teal}{I don't know}\\
\textbf{GPT-3.5}: \textcolor{purple}{degrees}\\
\colorbox{red!10}{\textbf{Irrelevant knowledge}:} Title: Inscribed angle\\
inscribed angle theorem states that an angle $\theta$ inscribed in a circle is half of the central angle 2$\theta$ that subtends the same arc on the circle. Therefore, the angle does not change as its vertex is moved to different positions on the circle...
\\
\midrule
\textbf{Question}: who played the colorado kid in rio bravo \\
\textbf{Reference answer}: Ricky Nelson\\
\textbf{Responses}: \\
\textbf{Alpaca}: \textcolor{purple}{The role of the Colorado Kid was played by John Dehner in the 1959 film Rio Bravo.}\\
\textbf{Flan-T5}: \textcolor{purple}{Jim J. Bullock}\\
\textbf{GPT-3.5}: \textcolor{teal}{I don't know.}\\
\colorbox{red!10}{\textbf{Irrelevant knowledge}:} Title: Jim J. Bullock\\
Jim J. Bullock James Jackson Bullock (born February 9, 1955), sometimes credited as Jm J. Bullock, is an American actor and comedian of stage, television and motion pictures... Bullock became a notable entertainment figure in the 1980s \\
\midrule

\textbf{Dataset}: HotpotQA \\
\\
% \textbf{Question}: Are both Elko Regional Airport and Gerald R. Ford International Airport located in Michigan?  \\
% \textbf{Reference answer}: no\\
% \textbf{Responses}:\\ 
% \textbf{Alpaca}: \textcolor{purple}{No, Elko Regional Airport is located in Elko, Nevada, and Gerald R. Ford International Airport is located in Grand Rapids, Michigan.}\\
% \textbf{Flan-T5}: \textcolor{purple}{no}\\
% \textbf{GPT-3.5}: \textcolor{teal}{I don't know}\\
% \colorbox{red!10}{\textbf{Irrelevant knowledge}:} Title: Elwood Airport\\
% Elwood Airport (FAA LID: 3I1) was a public use airport located two nautical miles (3.7km) south of the central business district of Elwood, in Madison County, Indiana, United States. The airfield closed on September 1, 2008.
% \\
% \midrule
\textbf{Question}: Ralph Hefferline was a psychology professor at a university that is located in what city? \\
\textbf{Reference answer}: New York City\\
\textbf{Responses}: \\
\textbf{Alpaca}: \textcolor{purple}{Columbia, Missouri.}\\
\textbf{Flan-T5}: \textcolor{purple}{Columbia}\\
\textbf{GPT-3.5}: \textcolor{teal}{I don't know.}\\
\colorbox{red!10}{\textbf{Irrelevant knowledge}:} Title: University of Missouri\\
The University of Missouri (also, Mizzou, or MU) is a public land-grant research university located in Columbia, Missouri, U.S. It was founded in 1839 ...
\\
\midrule
\textbf{Dataset}: TopiOCQA \\
\\
% \textbf{Question}: \\
% User: where may have the mycenaeans ultimately ended up\\
% Agent: Cyprus and the Levantine coast\\
% User: where is the former place located?\\
% \textbf{Reference answer}: In the Eastern Mediterranean, located south of Turkey; west of Syria and Lebanon; north of Egypt, Israel, and Palestine; and southeast of Greece.\\
% \textbf{Responses}:\\ 
% \textbf{Alpaca}: \textcolor{purple}{Cyprus is located in the Mediterranean Sea, south of Turkey, west of Syria and Lebanon, and north of Egypt.
% }\\
% \textbf{Flan-T5}: \textcolor{purple}{Cyprus}\\
% \textbf{GPT-3.5}: \textcolor{teal}{I don't know.}\\
% \colorbox{red!10}{\textbf{Irrelevant knowledge}:} Title: Ancient history of Cyprus\\
% Cyprus became a Roman province in 58 BCE. This came about, according to Strabo, because Publius Clodius Pulcher held a grudge against Ptolemy of Cyprus...
% \\
% \midrule
\textbf{Question}: \\
User: what is the location of mars in the solar system\\
Agent: Mars is the fourth planet from the Sun\\
User: is it known by any other names? \\
\textbf{Reference answer}: Red Planet\\
\textbf{Responses}: \\
\textbf{Alpaca}: \textcolor{purple}{No, it is known by its official name, Mars.}\\
\textbf{Flan-T5}: \textcolor{purple}{Mars is also known as the Red Planet.}\\
\textbf{GPT-3.5}: \textcolor{teal}{I don't know.}\\
\colorbox{red!10}{\textbf{Irrelevant knowledge}:} Title: Haboob\\
Global dust storms on Mars have been compared to haboobs on Earth.
\\
\bottomrule
\end{tabular}
\caption{Failure examples of the models in generating \emph{I don't know} in the presence of irrelevant knowledge.}\label{fig:unanswerability_irrelevant}
\end{figure*}

\begin{figure*}[ht!]
\small
\begin{tabular}{p{2\columnwidth}}
\toprule

\textbf{Dataset}: NQ \\
\\
\textbf{Question}: points on a sphere or angles in a circle are measured in units called \\
\textbf{Reference answer}: radians\\
\textbf{Responses}:\\ 
\textbf{Alpaca}: 1. \textcolor{teal}{radians}\\
\textbf{Flan-T5}: \textcolor{teal}{radians}\\
\textbf{GPT-3.5}: \textcolor{purple}{I don't know.}\\
\colorbox{green!10}{\textbf{Relevant knowledge}:} Title: Position angle\\
... It is calculated in a plane that contains the sphere center and the great circle, where is the angular distance of two points viewed from the center of the sphere, measured in \textbf{radians}...
\\
\midrule
\textbf{Question}: who had a baby at 100 in the bible \\
\textbf{Reference answer}: 1. Sarah, 2. Abraham\\
\textbf{Responses}:\\ 
\textbf{Alpaca}: 100 year old \textcolor{teal}{Sarah} had a baby with \textcolor{teal}{Abraham}.\\
\textbf{Flan-T5}: \textcolor{purple}{I don't know.}\\
\textbf{GPT-3.5}: \textcolor{teal}{Abraham} had a baby at 100 in the Bible.\\
\colorbox{green!10}{\textbf{Relevant knowledge}:} Title: The Bible and humor\\
... Macy says that in speaking of humor in the Bible he usually begins with asking how it might feel to personally get the message \textbf{Abraham and Sarah} received, putting them into the absurd situation of \textbf{a ninety year old having a baby}...
\\
\midrule

% \textbf{Question}: when did the isle of wight become an island \\
% \textbf{Reference answer}: During the last Ice Age\\
% \textbf{Responses}: \\
% \textbf{Alpaca}: 11,755 years ago, \textcolor{teal}{during the last ice age}, forming the Solent and turning Wight into an island. The Needles, along with Old Harry Rocks on Purbeck, represent the edges of this breach.\\
% \textbf{Flan-T5}: \textcolor{teal}{during the last ice age
% }\\
% \textbf{GPT-3.5}: \textcolor{purple}{I don't know.}\\
% \colorbox{green!10}{\textbf{Relevant knowledge}:} Title: Isle of Wight\\
% \textbf{during the last ice age}, forming the Solent and turning Wight into an island. The Needles, along with Old Harry Rocks on Purbeck, represent the edges of this breach...
% \\
% \toprule

\textbf{Dataset}: HotpotQA \\
\\
% \textbf{Question}: Are the Laleli Mosque and Esma Sultan Mansion located in the same neighborhood? \\
% \textbf{Reference answer}: no\\
% \textbf{Responses}:\\ 
% \textbf{Alpaca}: \textcolor{teal}{No}, they are not. The Laleli Mosque is located in the Fatih neighborhood of Istanbul, while the Esma Sultan Mansion is located in the Ortaköy\\
% \textbf{Flan-T5}: \textcolor{teal}{no}\\
% \textbf{GPT-3.5}: \textcolor{purple}{I don't know}\\
% \colorbox{green!10}{\textbf{Relevant knowledge}:} \\
% - Title: Laleli Mosque\\
% The Laleli Mosque (Turkish: "Laleli Camii, or Tulip Mosque" ) is an 18th-century Ottoman imperial mosque located in \textbf{Laleli, Fatih}, Istanbul, Turkey.\\
% - Title: Esma Sultan Mansion\\
% The Esma Sultan Mansion (Turkish: "Esma Sultan Yalısı" ), a historical yalı (English: waterside mansion ) located at Bosphorus in \textbf{Ortaköy neighborhood} of Istanbul, Turkey...
% \\
% \midrule
\textbf{Question}: Roger O. Egeberg was Assistant Secretary for Health and Scientific Affairs during the administration of a president that served during what years? \\
\textbf{Reference answer}: 1969 until 1974\\
\textbf{Responses}: \\
\textbf{Alpaca}: \textcolor{teal}{1969-1974.}\\
\textbf{Flan-T5}: \textcolor{teal}{1969 until 1974.}\\
\textbf{GPT-3.5}: \textcolor{purple}{I don't know.}\\
\colorbox{green!10}{\textbf{Relevant knowledge}:} \\
Title: Roger O. Egeberg\\
... His other roles included Assistant Secretary for Health and Scientific Affairs in the Department of Health, Education, and Welfare (now the United States Department of Health and Human Services) during the \textbf{Nixon administration} and Dean of the University of Southern California's medical school.\\
- Title: Richard Nixon\\
Richard Milhous Nixon (January 9, 1913 – April 22, 1994) was the 37th President of the United States \textbf{from 1969 until 1974}, ...\\
\midrule
\textbf{Dataset}: TopiOCQA \\
\\
% \textbf{Question}: \\
% User: where may have the mycenaeans ultimately ended up\\
% \textbf{Reference answer}: Cyprus and the Levantine coast\\
% \textbf{Responses}:\\ 
% \textbf{Alpaca}: The Mycenaeans ultimately ended up in a number of different places, including the Aegean islands, the Peloponnese, \textcolor{teal}{Cyprus, and the Levantine coast.}\\
% \textbf{Flan-T5}: Mycenaean refugees migrated to \textcolor{teal}{Cyprus and the Levantine coast.}\\
% \textbf{GPT-3.5}: \textcolor{purple}{I don't know.}\\
% \colorbox{green!10}{\textbf{Relevant knowledge}:} Title: Mycenaean Greece\\
% Mycenaean refugees migrated to Cyprus and the Levantine coast. Nevertheless, other regions on the edge of the Mycenaean world prospered, such as the Ionian islands, the northwestern Peloponnese, parts of Attica and a number of Aegean islands. The acropolis of Athens, oddly, appears to have avoided destruction.
% \\
% \midrule
\textbf{Question}: \\
User: how much did the blues brothers movie cost to make\\
\textbf{Reference answer}: \$17.5 million\\
\textbf{Responses}: \\
\textbf{Alpaca}: \textcolor{teal}{17.5 million}\\
\textbf{Flan-T5}: \textcolor{teal}{\$17.5 million}\\
\textbf{GPT-3.5}: \textcolor{purple}{I don't know.}\\
\colorbox{green!10}{\textbf{Relevant knowledge}:} Title: The Blues Brothers (film)\\
Principal photography began in July 1979, with the film's budget still not settled. For the first month, things ran smoothly on and off the set. When Weiss saw the supposedly final \textbf{\$17.5 million} budget, he reportedly joked, "I think we've spent that much already." ...
\\
\bottomrule
\end{tabular}
\caption{Failure examples of the models in generating informative responses in the presence of relevant knowledge.}\label{fig:unanswerability_relevant}
\end{figure*}
Results illustrated in \Cref{tab:unanswerability} show that models sometimes perform differently given relevant or irrelevant knowledge. \Cref{fig:unanswerability_irrelevant} demonstrates the failure examples of the studied models in all three QA datasets. It can be observed that given an irrelevant passage, models (especially Alpaca) do not refrain from answering. Moreover, failure examples presented in \Cref{fig:unanswerability_relevant} show that GPT-3.5 has difficulty in generating responses even when the correct information is available in the provided knowledge.
