# Supplementary material for: Evaluating Correctness and Faithfulness of Instruction-Following Models for Question Answering
Source: arXiv:2307.16877 source file (2024-04-17)
Supplement: Supplementary file 3 [file appendix_gpt4_failure_examples.tex]

\begin{figure*}[t]
\small
\begin{tabular}{p{2\columnwidth}}
\toprule
\textbf{Error Type:} Incomplete Reference Answers - Open-ended Questions\\
\textbf{Dataset}: TopiOCQA \\
\\
\textbf{Question}: does she (J.K. Rowling) donate to any charity? \\
\textbf{Reference answer}: Yes - In 2002, Rowling contributed a foreword to ``Magic'', an anthology of fiction published by Bloomsbury Publishing, helping to raise money for the National Council for One Parent Families. \\
\textbf{Alpaca's response}: Yes, she does. She is a member of both English PEN and Scottish PEN, and has donated the proceeds from several of her books to various charities.\\

\midrule

\textbf{Error Type:} Incomplete Reference Answers - List of Named Entities\\
\textbf{Dataset}: Natural Questions \\
\\
\textbf{Question}: what kind of animals live in the great victoria desert \\
\textbf{Reference answer}:  malleefowl; water-holding frog; great desert skink; sandhill dunnart; dingo; sand goanna; crest-tailed mulgara; southern marsupial mole; chestnut-breasted whiteface; perentie\\
\textbf{Flan-T5's response}: lizard.\\

\midrule

\textbf{Error Type:} Intrinsic Ambiguity in Questions\\
\textbf{Dataset}: Natural Questions \\
\\
\textbf{Question}: who played in the stanley cup finals last year\\
\textbf{Reference answers}: Nashville Predators, Pittsburgh Penguins\\
\textbf{GPT-3.5's response}: The Washington Capitals and the Vegas Golden Knights played in the Stanley Cup Finals last year (2018).\\
% clarifying question
% id 966
\bottomrule
\end{tabular}
\caption{Examples where GPT-4Eval predictions differ from human judgement (alongside $F_1<0.3$). %More details in \Cref{appendix_sec:gpt4-eval-failure}.
}
\label{fig:appendix_gpt4_failure_examples}
\end{figure*}
