# Supplementary material for: Evaluating Correctness and Faithfulness of Instruction-Following Models for Question Answering
Source: arXiv:2307.16877 source file (2024-04-17)
Supplement: Supplementary file 4 [file appendix.tex]

\appendix
% We should combine all of these appendices into a single file eventually.
% It will probably become cumbersome to managage labels.
\input{Sections/appendix_experimental_details}

% \input{Sections/appendix_prompts}

% \input{Sections/appendix_metric_failures}

% \input{Sections/appendix_gpt4_eval}

% \todo[]{

% (1) out of 296 cases, we filter out cases where GPT-4Eval = 0 and Humeval = 1, then divide those cases into the finegrained failure analysis. We only use the subcategories, not categories. We do a bar chart instead of a sunburst. THis will tell us where GPT4E will generally fail.

% (2) a few qualitative examples, which we can take from slides.

% (3) not much to talk about in this section, simply just mention the charts and examples.

% }

% \input{Sections/appendix_human_eval}

% \input{Sections/appendix_unanswerability}
