# Supplementary material for: Evaluating Correctness and Faithfulness of Instruction-Following Models for Question Answering
Source: arXiv:2307.16877 source file (2024-04-17)
Supplement: Supplementary file 5 [file appendix_correlation_ablation.tex]

\input{emnlp2023-latex/Tables/correlation_by_dataset}
\input{emnlp2023-latex/Tables/correlation_by_model}
\input{emnlp2023-latex/Tables/main_results_sample}
