# Supplementary material for: Evaluating Correctness and Faithfulness of Instruction-Following Models for Question Answering
Source: arXiv:2307.16877 source file (2024-04-17)
Supplement: Supplementary file 6 [file appendix_human_eval.tex]

\section{Human Evaluation}
\label{appendix_sec:human_eval}
\Cref{sec:correctness} and \Cref{sec:groundedness} describe the human evaluation procedures for both correctness of the responses w.r.t. information need and faithfulness of the models w.r.t. relevant knowledge.

\Cref{tab:main_results_100_sample} demonstrates the quantitative results on the 100 samples picked for human evaluation using all studied correctness metrics. 
Similarly, the faithfulness results on the 50 samples are presented in \Cref{tab:faithfulness_results_100_sample}.
