# Supplementary material for: Evaluating Correctness and Faithfulness of Instruction-Following Models for Question Answering
Source: arXiv:2307.16877 source file (2024-04-17)
Supplement: Supplementary file 7 [file appendix_prompts.tex]

\section{Prompts details}
\label{appendix_sec:prompts}

In \Cref{sec:correctness_metrics}, we introduce LLM-based evaluations to evaluate the correctness of a model response w.r.t. the user's information need. To accomplish this, we use the prompt template shown in \Cref{fig:prompt_correctness_eval}, and map ``yes'' to 1 and ``no'' to 0. Similarly, \Cref{paragraph:llm_critic_eval_groundedness} introduces the LLMCritic Evaluation method for calculating the faithfulness of the models w.r.t. relevant knowledge. To run this evaluation, we used the prompt shown in \Cref{fig:prompt_faithfulness_eval}.

Furthermore, we conducted other experiments to study the answer abstience of the models in \Cref{sec:unanswerability}. The template used in these experiments is shown in \Cref{fig:prompt_unanswerability}.
